# Supplementary material for: Perturbation theory without power series: iterative construction of non-analytic operator spectra
Source: arXiv:2105.04972 source file (2022-10-27)
Supplement: Supplementary file 1 [file SI.pdf]

# Supplementary Material:
# Relaxed perturbation theory: iterative construction of non-analytic spectra without resummation

Matteo Smerlak

*Max Planck Institute for Mathematics in the Sciences, Leipzig, Germany*

## I. RELAXED PERTUBATION THEORY: A TOY EXAMPLE

To build intuition for the difference between relaxed RS and IPT theories on the one hand, and conventional perturbative expansions on the other hand, it is useful to consider the simple two-dimensional Hamiltonian

$$H = H_0 + H_1 \quad \text{with} \quad H_0 = \begin{pmatrix} 0 & 0 \\ 0 & 1 \end{pmatrix} \quad \text{and} \quad H_1 = \begin{pmatrix} 0 & g \\ g & 0 \end{pmatrix}. \tag{S1}$$

This matrix has ground state energy $E(g) = (1 - \sqrt{1+4g^2})/2$. At the exceptional points $g = \pm i/2$, this function has branch-point singularities which signal that $H$ is no longer diagonalizable. Consequently, the conventional RS expansion of $E(g)$ can only converge in a centered disk $D_{1/2}$ with radius 1/2, although $E(g)$ is analytic everywhere except at $g = \pm i/2$. Let us now examine how relaxed perturbation theory behaves in this case.

*Relaxed IPT.* The simpler case to analyze is IPT. For the ground state we have

$$\psi^{(k)}_{\mathrm{IPT}} = \begin{pmatrix} 1 \\ q_\alpha^k(0) \end{pmatrix} \quad \text{with} \quad q_\alpha(x) = \alpha g(x^2-1) + (1-\alpha)x. \tag{S2}$$

Here the superscript denotes $k$-fold composition. Evaluated at its fixed point $x_* = (1 - \sqrt{1+4g^2})/2g$, the Jacobian of $q_\alpha$ reads $q'_\alpha(x_*) = 1 - \alpha\sqrt{1+4g^2}$. This quantity has modulus smaller than 1 inside a cardioid-shape domain in the complex plane, which is therefore the domain of convergence of IPT. This domain excludes the singular points $\pm i/2$, but extends along the real axis up to arbitrarily large values of $g$ for sufficiently small $\alpha$. For $\alpha = 1$ (no relaxation), this domain is strictly greater than the disk $D_{1/2}$.

*Relaxed RS theory.* The RS expansion of the ground state with $\alpha$-relaxation to $k$-th order reads [S1]

$$\psi^{(k)}_{\mathrm{RS}} = \sum_{l=0}^{k} \sum_{s=1}^{l} \binom{l-1}{s-1} \alpha^s (1-\alpha)^{l-s} g^s a_s \tag{S3}$$

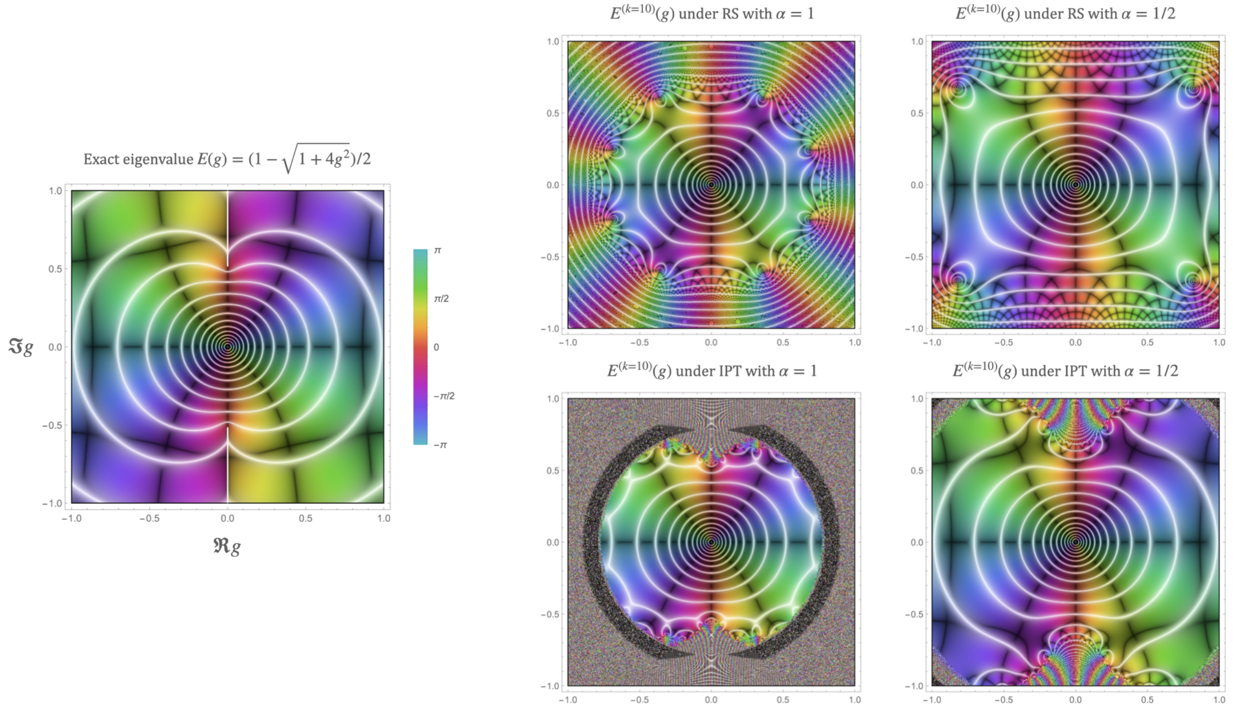


FIG. S1. Different ways to construct a complex function with singularities with polynomials. In all plots color indicates argument, brightness indicates log-modulus, and saturation indicates real and imaginary magnitude. Left: Left: The exact eigenvalue $E(g) = (1 - \sqrt{1+4g^2})/2$, with its branch-point singularities at $g = \pm i/2$. Its Taylor expansion in $g$ must diverge outside the disk $D_{1/2}$ with radius $1/2$. Right, top row: the conventional RS series ($\alpha = 1$) is valid inside a circle with radius $1/2$, but the same expansion with $\alpha = 1/2$ has a larger, non-circular domain of convergence. Right, bottom row: IPT with $\alpha = 1$ converges inside a cardioid shaped domain which is stricly larger than $D_{1/2}$; with $\alpha = 1/2$ this domain extends yet further.

where $a_s$ are the coefficients of the standard (unrelaxed) RS expansion of $\psi$. This expression is not a power series in $g$, hence its domain of convergence is not restricted to the disk $D_{1/2}$.

Fig. S1 illustrates these constructions graphically. From this figure it is apparent that, at least in this simple case, IPT at a given order $k = 10$ approximates $E(g)$ better than RS theory at the same order, and that in both cases $\alpha = 1/2$ provides extended convergence with respect to the $\alpha = 1$.

## II. PYTHON CODE FOR IPT-AA

```python
import aa # Anderson acceleration from https://github.com/cvxgrp/aa

import numpy as np
import time

def eigs_ipt(H, i = 0, v0 = None, mem = 10, maxiter = 1000, tol = 1e-10):

    dim = H.shape[0]
    H0 = H.diagonal()  # Epstein-Nesbet partitioning
    g = H0[i] - H0; g[i]=1; R0 = 1/g; R0[i] = 0  # Reduced resolvent
    aa_wrk = aa.AndersonAccelerator(dim, mem)    # Initialize accelerator
    e = np.zeros(dim); e[i] = 1  # Unperturbed eigenvector (basis state)
    if v0 is not None:
        w = v0
    else:
        w = e

    def Q(v, R0, H0):    # Quadratic operator, eq. (3) in main text
        H1v = H @ v - np.multiply(H0, v)
        return(e + np.multiply(R0, H1v - H1v[i]*v), H1v)

    err = [1]
    l = 0

    tic = time.time()
    while l <= maxiter and err[-1]>tol:
        v = w
        w, H1v = Q(v, R0, H0)  # Iterate Q
        l += 1
        aa_wrk.apply(w, v) # Anderson acceleration
        E = H0[i] + H1v[i] # Evaluate energy
        err.append(np.linalg.norm(v - w)) # Estimate error
    toc = time.time()

    print('Iterations:', l - 1)
    print('Time:', toc - tic)

    return(E, v)
```

[S1] C. Schmidt, M. Warken, and N. C. Handy, Chemical physics letters **211**, 272 (1993).
